# Supplementary material for: Rethinking the Relationship between Recurrent and Non-Recurrent Neural Networks: A Study in Sparsity
Source: arXiv:2404.00880 source file (2024-04-01)
Supplement: Supplementary file 1 [file appendix.tex]

\begin{figure}
\centering
\includegraphics[width=0.4\textwidth]{figures/Training vs Validation RNN medium last.pdf}
\caption{Training vs Validation RNN medium last}
\label{fig:Training vs Validation RNN medium last}
\end{figure}

\begin{figure}
\centering
\includegraphics[width=0.4\textwidth]{figures/Training vs Validation sequential2D_MLP medium last.pdf}
\caption{Training vs Validation sequential2D\_MLP medium last}
\label{fig:Training vs Validation sequential2D_MLP medium last}
\end{figure}

\begin{figure}
\centering
\includegraphics[width=0.4\textwidth]{figures/Training vs Validation sequential2D_dense medium last.pdf}
\caption{Training vs Validation sequential2D\_dense medium last}
\label{fig:Training vs Validation sequential2D_dense medium last}
\end{figure}

\begin{figure}
\centering
\includegraphics[width=0.4\textwidth]{figures/Training vs Validation sequential2D_sparse medium last.pdf}
\caption{Training vs Validation sequential2D\_sparse medium last}
\label{fig:Training vs Validation sequential2D_sparse medium last}
\end{figure}

\begin{figure}
\centering
\includegraphics[width=0.4\textwidth]{figures/Training vs Validation RNN medium all.pdf}
\caption{Training vs Validation RNN medium all}
\label{fig:Training vs Validation RNN medium all}
\end{figure}

\begin{figure}
\centering
\includegraphics[width=0.4\textwidth]{figures/Training vs Validation sequential2D_MLP medium all.pdf}
\caption{Training vs Validation sequential2D\_MLP medium all}
\label{fig:Training vs Validation sequential2D_MLP medium all}
\end{figure}

\begin{figure}
\centering
\includegraphics[width=0.4\textwidth]{figures/Training vs Validation sequential2D_dense medium all.pdf}
\caption{Training vs Validation sequential2D\_dense medium all}
\label{fig:Training vs Validation sequential2D_dense medium all}
\end{figure}

\begin{figure}
\centering
\includegraphics[width=0.4\textwidth]{figures/Training vs Validation sequential2D_sparse medium all.pdf}
\caption{Training vs Validation sequential2D\_sparse medium all}
\label{fig:Training vs Validation sequential2D_sparse medium all}
\end{figure}

\begin{figure}
\centering
\includegraphics[width=0.4\textwidth]{figures/Training vs Validation RNN both_uniform last.pdf}
\caption{Training vs Validation RNN both\_uniform last}
\label{fig:Training vs Validation RNN both_uniform last}
\end{figure}

\begin{figure}
\centering
\includegraphics[width=0.4\textwidth]{figures/Training vs Validation sequential2D_MLP both_uniform last.pdf}
\caption{Training vs Validation sequential2D\_MLP both\_uniform last}
\label{fig:Training vs Validation sequential2D_MLP both_uniform last}
\end{figure}

\begin{figure}
\centering
\includegraphics[width=0.4\textwidth]{figures/Training vs Validation sequential2D_dense both_uniform last.pdf}
\caption{Training vs Validation sequential2D\_dense both\_uniform last}
\label{fig:Training vs Validation sequential2D_dense both_uniform last}
\end{figure}

\begin{figure}
\centering
\includegraphics[width=0.4\textwidth]{figures/Training vs Validation sequential2D_sparse both_uniform last.pdf}
\caption{Training vs Validation sequential2D\_sparse both\_uniform last}
\label{fig:Training vs Validation sequential2D_sparse both_uniform last}
\end{figure}

\begin{figure}
\centering
\includegraphics[width=0.4\textwidth]{figures/Training vs Validation RNN both_uniform all.pdf}
\caption{Training vs Validation RNN both\_uniform all}
\label{fig:Training vs Validation RNN both_uniform all}
\end{figure}

\begin{figure}
\centering
\includegraphics[width=0.4\textwidth]{figures/Training vs Validation sequential2D_MLP both_uniform all.pdf}
\caption{Training vs Validation sequential2D\_MLP both\_uniform all}
\label{fig:Training vs Validation sequential2D_MLP both_uniform all}
\end{figure}

\begin{figure}
\centering
\includegraphics[width=0.4\textwidth]{figures/Training vs Validation sequential2D_dense both_uniform all.pdf}
\caption{Training vs Validation sequential2D\_dense both\_uniform all}
\label{fig:Training vs Validation sequential2D_dense both_uniform all}
\end{figure}

\begin{figure}
\centering
\includegraphics[width=0.4\textwidth]{figures/Training vs Validation sequential2D_sparse both_uniform all.pdf}
\caption{Training vs Validation sequential2D\_sparse both\_uniform all}
\label{fig:Training vs Validation sequential2D_sparse both_uniform all}
\end{figure}

\begin{figure}
\centering
\includegraphics[width=0.4\textwidth]{figures/Training vs Validation RNN both_random last.pdf}
\caption{Training vs Validation RNN both\_random last}
\label{fig:Training vs Validation RNN both_random last}
\end{figure}

\begin{figure}
\centering
\includegraphics[width=0.4\textwidth]{figures/Training vs Validation sequential2D_MLP both_random last.pdf}
\caption{Training vs Validation sequential2D\_MLP both\_random last}
\label{fig:Training vs Validation sequential2D_MLP both_random last}
\end{figure}

\begin{figure}
\centering
\includegraphics[width=0.4\textwidth]{figures/Training vs Validation sequential2D_dense both_random last.pdf}
\caption{Training vs Validation sequential2D\_dense both\_random last}
\label{fig:Training vs Validation sequential2D_dense both_random last}
\end{figure}

\begin{figure}
\centering
\includegraphics[width=0.4\textwidth]{figures/Training vs Validation sequential2D_sparse both_random last.pdf}
\caption{Training vs Validation sequential2D\_sparse both\_random last}
\label{fig:Training vs Validation sequential2D_sparse both_random last}
\end{figure}

\begin{figure}
\centering
\includegraphics[width=0.4\textwidth]{figures/Training vs Validation RNN both_random all.pdf}
\caption{Training vs Validation RNN both\_random all}
\label{fig:Training vs Validation RNN both_random all}
\end{figure}

\begin{figure}
\centering
\includegraphics[width=0.4\textwidth]{figures/Training vs Validation sequential2D_MLP both_random all.pdf}
\caption{Training vs Validation sequential2D\_MLP both\_random all}
\label{fig:Training vs Validation sequential2D_MLP both_random all}
\end{figure}

\begin{figure}
\centering
\includegraphics[width=0.4\textwidth]{figures/Training vs Validation sequential2D_dense both_random all.pdf}
\caption{Training vs Validation sequential2D\_dense both\_random all}
\label{fig:Training vs Validation sequential2D_dense both_random all}
\end{figure}

\begin{figure}
\centering
\includegraphics[width=0.4\textwidth]{figures/Training vs Validation sequential2D_sparse both_random all.pdf}
\caption{Training vs Validation sequential2D\_sparse both\_random all}
\label{fig:Training vs Validation sequential2D_sparse both_random all}
\end{figure}

\begin{figure}
\centering
\includegraphics[width=0.4\textwidth]{figures/model validation comparison medium last.pdf}
\caption{model validation comparison medium last}
\label{fig:model validation comparison medium last}
\end{figure}

\begin{figure}
\centering
\includegraphics[width=0.4\textwidth]{figures/model validation comparison both_uniform last.pdf}
\caption{model validation comparison both\_uniform last}
\label{fig:model validation comparison both_uniform last}
\end{figure}

\begin{figure}
\centering
\includegraphics[width=0.4\textwidth]{figures/model validation comparison both_random last.pdf}
\caption{model validation comparison both\_random last}
\label{fig:model validation comparison both_random last}
\end{figure}

\begin{figure}
\centering
\includegraphics[width=0.4\textwidth]{figures/model validation comparison medium all.pdf}
\caption{model validation comparison medium all}
\label{fig:model validation comparison medium all}
\end{figure}

\begin{figure}
\centering
\includegraphics[width=0.4\textwidth]{figures/model validation comparison both_uniform all.pdf}
\caption{model validation comparison both\_uniform all}
\label{fig:model validation comparison both_uniform all}
\end{figure}

\begin{figure}
\centering
\includegraphics[width=0.4\textwidth]{figures/model validation comparison both_random all.pdf}
\caption{model validation comparison both\_random all}
\label{fig:model validation comparison both_random all}
\end{figure}

\begin{figure}
\centering
\includegraphics[width=0.4\textwidth]{figures/iteration comparison medium RNN last.pdf}
\caption{iteration comparison medium RNN last}
\label{fig:iteration comparison medium RNN last}
\end{figure}

\begin{figure}
\centering
\includegraphics[width=0.4\textwidth]{figures/iteration comparison medium RNN all.pdf}
\caption{iteration comparison medium RNN all}
\label{fig:iteration comparison medium RNN all}
\end{figure}

\begin{figure}
\centering
\includegraphics[width=0.4\textwidth]{figures/iteration comparison medium sequential2D_MLP last.pdf}
\caption{iteration comparison medium sequential2D\_MLP last}
\label{fig:iteration comparison medium sequential2D_MLP last}
\end{figure}

\begin{figure}
\centering
\includegraphics[width=0.4\textwidth]{figures/iteration comparison medium sequential2D_MLP all.pdf}
\caption{iteration comparison medium sequential2D\_MLP all}
\label{fig:iteration comparison medium sequential2D_MLP all}
\end{figure}

\begin{figure}
\centering
\includegraphics[width=0.4\textwidth]{figures/iteration comparison medium sequential2D_dense last.pdf}
\caption{iteration comparison medium sequential2D\_dense last}
\label{fig:iteration comparison medium sequential2D_dense last}
\end{figure}

\begin{figure}
\centering
\includegraphics[width=0.4\textwidth]{figures/iteration comparison medium sequential2D_dense all.pdf}
\caption{iteration comparison medium sequential2D\_dense all}
\label{fig:iteration comparison medium sequential2D_dense all}
\end{figure}

\begin{figure}
\centering
\includegraphics[width=0.4\textwidth]{figures/iteration comparison medium sequential2D_sparse last.pdf}
\caption{iteration comparison medium sequential2D\_sparse last}
\label{fig:iteration comparison medium sequential2D_sparse last}
\end{figure}

\begin{figure}
\centering
\includegraphics[width=0.4\textwidth]{figures/iteration comparison medium sequential2D_sparse all.pdf}
\caption{iteration comparison medium sequential2D\_sparse all}
\label{fig:iteration comparison medium sequential2D_sparse all}
\end{figure}

\begin{figure}
\centering
\includegraphics[width=0.4\textwidth]{figures/all vs last medium RNN.pdf}
\caption{all vs last medium RNN}
\label{fig:all vs last medium RNN}
\end{figure}

\begin{figure}
\centering
\includegraphics[width=0.4\textwidth]{figures/all vs last medium sequential2D_MLP.pdf}
\caption{all vs last medium sequential2D\_MLP}
\label{fig:all vs last medium sequential2D_MLP}
\end{figure}

\begin{figure}
\centering
\includegraphics[width=0.4\textwidth]{figures/all vs last medium sequential2D_dense.pdf}
\caption{all vs last medium sequential2D\_dense}
\label{fig:all vs last medium sequential2D_dense}
\end{figure}

\begin{figure}
\centering
\includegraphics[width=0.4\textwidth]{figures/all vs last medium sequential2D_sparse.pdf}
\caption{all vs last medium sequential2D\_sparse}
\label{fig:all vs last medium sequential2D_sparse}
\end{figure}

\begin{figure}
\centering
\includegraphics[width=0.4\textwidth]{figures/all vs last both_uniform RNN.pdf}
\caption{all vs last both\_uniform RNN}
\label{fig:all vs last both_uniform RNN}
\end{figure}

\begin{figure}
\centering
\includegraphics[width=0.4\textwidth]{figures/all vs last both_uniform sequential2D_MLP.pdf}
\caption{all vs last both\_uniform sequential2D\_MLP}
\label{fig:all vs last both_uniform sequential2D_MLP}
\end{figure}

\begin{figure}
\centering
\includegraphics[width=0.4\textwidth]{figures/all vs last both_uniform sequential2D_dense.pdf}
\caption{all vs last both\_uniform sequential2D\_dense}
\label{fig:all vs last both_uniform sequential2D_dense}
\end{figure}

\begin{figure}
\centering
\includegraphics[width=0.4\textwidth]{figures/all vs last both_uniform sequential2D_sparse.pdf}
\caption{all vs last both\_uniform sequential2D\_sparse}
\label{fig:all vs last both_uniform sequential2D_sparse}
\end{figure}

\begin{figure}
\centering
\includegraphics[width=0.4\textwidth]{figures/all vs last both_random RNN.pdf}
\caption{all vs last both\_random RNN}
\label{fig:all vs last both_random RNN}
\end{figure}

\begin{figure}
\centering
\includegraphics[width=0.4\textwidth]{figures/all vs last both_random sequential2D_MLP.pdf}
\caption{all vs last both\_random sequential2D\_MLP}
\label{fig:all vs last both_random sequential2D_MLP}
\end{figure}

\begin{figure}
\centering
\includegraphics[width=0.4\textwidth]{figures/all vs last both_random sequential2D_dense.pdf}
\caption{all vs last both\_random sequential2D\_dense}
\label{fig:all vs last both_random sequential2D_dense}
\end{figure}

\begin{figure}
\centering
\includegraphics[width=0.4\textwidth]{figures/all vs last both_random sequential2D_sparse.pdf}
\caption{all vs last both\_random sequential2D\_sparse}
\label{fig:all vs last both_random sequential2D_sparse}
\end{figure}
