# Supplementary material for: Rethinking the Relationship between Recurrent and Non-Recurrent Neural Networks: A Study in Sparsity
Source: arXiv:2404.00880 source file (2024-04-01)
Supplement: Supplementary file 2 [file appendix_diagonal.tex]

\subsection{Diagonal blocks} \label{sec:appendix-diagonal}

Let
\begin{equation}\label{eq:generalizations-diagonal}
M_{d4} = 
  \left[
      \begin{matrix}
  \Wy{I} & 0 & 0 & 0\\
  \myfone & \Wy{S} & 0 & 0\\
  0 & \myftwo & 0 & 0\\
  0 & 0 & \myfthr & 0
      \end{matrix}
    \right]
  \end{equation}
Note that after three iterations
  \begin{equation} \label{eq:generalizations-diagonal-M3-iteration3}
    \circ_{i=1}^3 M_{d}  
      \begin{bmatrix}
          \mv{h}_0 \\
          0 \\
          0 \\
          0 \\
      \end{bmatrix}
 = 
      \begin{bmatrix}
  \mv{h}_0 \\
  \myfone \circ \mv{h}_0 + \Wy{S} \circ \myfone \circ \mv{h}_0 +  \Wy{S} \circ \Wy{S} \circ \myfone \circ \mv{h}_0 \\
  \myftwo \circ \myfone \circ \mv{h}_0 + \myftwo \circ \Wy{S} \circ \myfone \circ \mv{h}_0 \\
  \myfthr \circ \myftwo \circ \myfone \circ \mv{h}_0 
      \end{bmatrix}
  \end{equation}
After four iterations
  \begin{equation} \label{eq:generalizations-diagonal-M3-iteration4}
    \circ_{i=1}^4 M_{d}  
      \begin{bmatrix}
         \mv{h}_0 \\
          0 \\
          0 \\
          0 \\
      \end{bmatrix}
  = 
      \begin{bmatrix}
  \mv{h}_0 \\
  \Wy{S} \circ \myfone \circ \mv{h}_0 +  \Wy{S} \circ \Wy{S} \circ \myfone \circ \mv{h}_0 +  \Wy{S} \circ \Wy{S} \circ \Wy{S} \circ \myfone \circ \mv{h}_0 +  \myfone \circ \mv{h}_0 \\
  \myftwo \circ \Wy{S} \circ \myfone \circ \mv{h}_0 +  \myftwo \circ \Wy{S} \circ \Wy{S} \circ \myfone \circ \mv{h}_0 +  \myftwo \circ \myfone \circ \mv{h}_0 \\
  \myfthr \circ \myftwo \circ \Wy{S} \circ \myfone \circ \mv{h}_0 +  \myfthr \circ \myftwo \circ \myfone \circ \mv{h}_0 
      \end{bmatrix}
  \end{equation}
In general, after the $k$-th iteration, if $S$ and $f_{\theta_i}$ are linear, with $k \ge 3$ we have
  \begin{equation} \label{eq:generalizations-diagonal-M3-iterationk}
    \circ_{i=1}^k M_{d}  
      \begin{bmatrix}
          \mv{h}_0 \\
          0 \\
          0 \\
          0 \\
      \end{bmatrix}
 = 
      \begin{bmatrix}
  \mv{h}_0 \\
  ( \circ_{i=0}^{k-1} \Wy{S} ) \circ \myfone \circ \mv{h}_0 \\
  \myftwo \circ ( \circ_{i=0}^{k-2} \Wy{S} ) \circ \myfone \circ \mv{h}_0 \\
  \myfthr \circ \myftwo \circ ( \circ_{i=0}^{k-3} \Wy{S} ) \circ \myfone \circ \mv{h}_0 
      \end{bmatrix}
  \end{equation}

So, in the linear case, the convergence of the above as $k \longmapsto \infty$ is determined by the convergence of the infinite product of $S$ alone, i.e., if we choose $S$ \emph{and} the $f_{\theta_j}$ to be a linear function  where the power-series is well understood.

\subsubsection{\tblue{Choice of the initial vector}}\label{sec:appendix-diagonal-q}

\tblue{The iteration will {\bf not} be independent of the initial vector}

Note that after three iterations
  \begin{equation} \label{eq:generalizations-diagonal-M3-iteration3}
    \circ_{i=1}^3 M_{d}  
      \begin{bmatrix}
          \mv{h}_0 \\
          q_1 \\
          q_2 \\
          q_3 \\
      \end{bmatrix}
 = 
      \begin{bmatrix}
  \mv{h}_0 \\
  \myfone \circ \mv{h}_0  + \Wy{S} \circ \myfone \circ \mv{h}_0 +  \Wy{S} \circ \Wy{S} \circ \myfone \circ \mv{h}_0 + \Wy{S} \circ \Wy{S} \circ \Wy{S} \circ q_1  \\
  \myftwo \circ \myfone \circ \mv{h}_0  + \myftwo \circ \Wy{S} \circ \myfone \circ \mv{h}_0 +  \myftwo \circ \Wy{S} \circ \Wy{S} \circ q_1 \\
  \myfthr \circ \myftwo \circ \myfone \circ \mv{h}_0 + \myfthr \circ \myftwo \circ \Wy{S} \circ q_1 
      \end{bmatrix}
  \end{equation}
