# Supplementary material for: Rethinking the Relationship between Recurrent and Non-Recurrent Neural Networks: A Study in Sparsity
Source: arXiv:2404.00880 source file (2024-04-01)
Supplement: Supplementary file 3 [file appendix_epsilonI.tex]

\subsection{Arbitrarily close to finite impulse response maps}
Now consider 
\begin{equation} \label{eq:appendix-Minfty-epsilon}
    M_{\infty}(\epsilon) =
    \begin{bmatrix}
        \epsilon \Wy{I}   & 0                 & 0                 & 0 \\
        \Wg{f_{\theta_1}}          & 0                 & 0                 & 0 \\
        0                 & \Wg{f_{\theta_2}}          & 0                 & 0 \\
        0                 & 0                 & \Wg{f_{\theta_3}}          & 0 \\
    \end{bmatrix}.
\end{equation}
where $0 \le \epsilon \le 1$ which as $\epsilon \rightarrow 0$ becomes arbitrarily close to a finite impulse response map.  In fact, it is exactly an finite impulse response map when $\epsilon=0$ and an infinite impulse response map when $\epsilon=1$. Defining
\begin{equation} \label{eq:SKIP_Minfty_epsilon_k}
    \circ_{i=1}^k M_{\infty}(\epsilon) = M_{\infty}(\epsilon) \circ M_{\infty}(\epsilon) \circ \dots \circ M_{\infty}(\epsilon) 
\end{equation}
for any value of $\epsilon$ after three iterations, 
\begin{equation} \label{eq:appendix-Minfty-epsilon-3}
    \circ_{i=1}^3 M_{\infty}(\epsilon) = 
    M_{\infty}(\epsilon) \circ 
    M_{\infty}(\epsilon) \circ 
    M_{\infty}(\epsilon) \circ 
    \begin{bmatrix}
        \mv{h}_0 \\
        0 \\
        0 \\
        0 \\
    \end{bmatrix} 
    = \begin{bmatrix}
        \epsilon^3 \mv{h}_0 \\
        \Wg{f_{\theta_1}}(\epsilon^2 \mv{h}_0) \\
        \Wg{f_{\theta_2}}(\Wg{f_{\theta_1}}(\epsilon \mv{h}_0)) \\
        \Wg{f_{\theta_3}}(\Wg{f_{\theta_2}}(\Wg{f_{\theta_1}}(\mv{h}_0)))  \\
    \end{bmatrix}
\end{equation}.
After four iterations,
\begin{equation} \label{eq:appendix-Minfty-epsilon-4}
    \circ_{i=1}^4 M_{\infty}(\epsilon) =
    M_{\infty}(\epsilon) \circ 
    M_{\infty}(\epsilon) \circ 
    M_{\infty}(\epsilon) \circ 
    M_{\infty}(\epsilon) \circ 
    \begin{bmatrix}
        \mv{h}_0 \\
        0 \\
        0 \\
        0 \\
    \end{bmatrix} 
    = \begin{bmatrix}
        \epsilon^4 \mv{h}_0 \\
        \Wg{f_{\theta_1}}(\epsilon^3 \mv{h}_0) \\
        \Wg{f_{\theta_2}}(\Wg{f_{\theta_1}}(\epsilon^2 \mv{h}_0)) \\
        \Wg{f_{\theta_3}}(\Wg{f_{\theta_2}}(\Wg{f_{\theta_1}}(\epsilon \mv{h}_0)))  \\
    \end{bmatrix}
\end{equation}
Further,
\begin{equation} \label{eq:appendix-Minfty-epsilon-k}
    \circ_{i=1}^k M_{\infty}(\epsilon) 
    \begin{bmatrix}
        \mv{h}_0 \\
        0 \\
        0 \\
        0 \\
    \end{bmatrix}
    = \begin{bmatrix}
        \epsilon^k \mv{h}_0 \\
        \Wg{f_{\theta_1}}(\epsilon^{k-1} \mv{h}_0) \\
        \Wg{f_{\theta_2}}(\Wg{f_{\theta_1}}(\epsilon^{k-2} \mv{h}_0)) \\
        \Wg{f_{\theta_3}}(\Wg{f_{\theta_2}}(\Wg{f_{\theta_1}}(\epsilon^{k-3} \mv{h}_0)))  \\
    \end{bmatrix}
\end{equation}
hence if it \emph{converges} to a finite impulse map when $\epsilon \rightarrow 0$ and $f_{\theta_i}=0, \forall i=1, 2, 3$. Further, for $0 < \epsilon < 1$ converges \emph{asymptotically} to a finite impulse map as $k \rightarrow \infty$ and $f_{\theta_i}=0, \forall i=1, \dots, k$. We conclude there is a \emph{continuum}, parametrized by $\epsilon$ between a finite impulse response map, and a response map whose impulse response approaches zero \emph{asymptotically}, and a recurrent neural network with infinite (non-converging) impulse response.
