# Supplementary material for: Rethinking the Relationship between Recurrent and Non-Recurrent Neural Networks: A Study in Sparsity
Source: arXiv:2404.00880 source file (2024-04-01)
Supplement: Supplementary file 4 [file appendix_generalizations.tex]

\section{Appendix} 
\label{sec:generalizations}

\subsection{Generalizations} \label{sec:sequential2D}
\todo{This section needs to be cleaned up.  There are twp versions of the same thing.  Use the colored one, but keep the points from the earlier one.}
% \begin{definition} \label{defn:seqential2D}
% Sequential2D is a rectangular block matrix function within which each entry is a matrix function. A Sequential2D map is of the form
% \begin{equation} \label{eq:Sequential2D}
%     M = \begin{bmatrix} D_{11} &A_{12}  &\hdots &A_{1n}  \\
%                         A_{21} &D_{22} &\hdots &A_{2n}  \\
%                         \vdots &       &\ddots &\vdots \\
%                         A_{n1} &A_{n2} &\hdots &D_{nn}
%         \end{bmatrix}                    
% \end{equation}
% where at least one of $A_{ij}, i \not= j$ is non-zero.
% By contrast Sequential1D maps are a subset of Sequential2D maps of the form
% \begin{equation} \label{eq:Sequential1D}
%     M = \begin{bmatrix} D_{11} &0      &\hdots  &0  \\
%                         D_{22} &0      &\hdots  &0  \\
%                         \vdots &\vdots &\ddots  &\vdots \\
%                         D_{nn} &0      &\hdots  &0
%         \end{bmatrix}                    
% \end{equation}

% \end{definition}
% In many ways, \eqref{eq:Sequential2D} is a straightforward generalization of a block-defined matrix.  In particular, if every function $A_{ij}$ happened to be linear (i.e., a matrix) and the function composition operator $\circ$ were replaced with the dot-product, then \eqref{eq:Sequential2D} would be precisely a block defined matrix. 

TBD TBD TBD TBD TBD TBD TBD TBD
TBD TBD TBD TBD TBD TBD TBD TBD
TBD TBD TBD TBD TBD TBD TBD TBD
TBD TBD TBD TBD TBD TBD TBD TBD
TBD TBD TBD TBD TBD TBD TBD TBD
TBD TBD TBD TBD TBD TBD TBD TBD
TBD TBD TBD TBD TBD TBD TBD TBD
TBD TBD TBD TBD TBD TBD TBD TBD
TBD TBD TBD TBD TBD TBD TBD TBD
TBD TBD TBD TBD TBD TBD TBD TBD
TBD TBD TBD TBD TBD TBD TBD TBD
TBD TBD TBD TBD TBD TBD TBD TBD
This opens an entire range of new possibilities when considering a block iterative function of the form

% Full matrix
\begin{equation} \label{eq:generalizations-full}
    \begin{bmatrix}
        \Wy{W_{1,1}} & \Wr{W_{1,2}}  & \Wr{W_{1,3}}  & \Wr{W_{1,4}}  & \Wr{W_{1,5}} \\
        \Wg{W_{2,1}} & \Wy{W_{2,2}}  & \Wr{W_{2,3}}  & \Wr{W_{2,4}}  & \Wr{W_{2,5}} \\
        \Wb{W_{3,1}} & \Wg{W_{3,2}}  & \Wy{W_{3,3}}  & \Wr{W_{3,4}}  & \Wr{W_{3,5}} \\
        \Wb{W_{4,1}} & \Wb{W_{4,2}}  & \Wg{W_{4,3}}  & \Wy{W_{4,4}}  & \Wr{W_{4,5}} \\
        \Wb{W_{5,1}} & \Wb{W_{5,2}}  & \Wb{W_{5,3}}  & \Wg{W_{5,4}}  & \Wy{W_{5,5}} \\
    \end{bmatrix}
\end{equation}

In this notation, 
\begin{itemize}
\item $\Wr{W_{i-k,i}}, \; k>1$ corresponds to TBD TBD TBD TBD TBD TBD TBD TBD TBD TBD TBD TBD TBD TBD TBD.
\item $\Wy{W_{i,i}}$ corresponds to TBD TBD TBD TBD TBD TBD TBD TBD TBD TBD TBD TBD TBD TBD TBD.
\item $\Wg{W_{i+1,i}}$ corresponds to a standard MLP or, more generally, an NN that can be implemented as a Pytorch or Keras Sequential container.
\item $\Wb{W_{i+k,i}}, \; k>1$ corresponds to skip connections and finite impulse response (FIR) filters.
%\item We began the exploration of $\Wy{W_{i,i}}$ with the introduction of the $I$ in \eqref{FIXME} corresponds infinite impulse response filters.
%\item What do $\Wr{W_{i,j}}, \; j>i$ correspond to?  They are actually \emph{feedback} connections which also lead to infinite impulse response filters and classic RNNs.
\end{itemize}
