# Supplementary material for: Rethinking the Relationship between Recurrent and Non-Recurrent Neural Networks: A Study in Sparsity
Source: arXiv:2404.00880 source file (2024-04-01)
Supplement: Supplementary file 5 [file appendix_skip.tex]

\subsection{Subdiagonal blocks - aka skip connections} \label{sec:appendix-skip-connections}

Define
\begin{equation} \label{eq:skip-connections}
    SK(\eta)=
    \begin{bmatrix}
        \Wy{I}        & 0                 & 0        & 0 \\
        \Wg{f_{\theta_1}}      & 0                 & 0        & 0 \\
        0             & \Wg{f_{\theta_2}}          & 0        & 0 \\
        \eta\Wb{S}    & 0                 & \Wg{f_{\theta_3}} & 0 \\
    \end{bmatrix}.
\end{equation}
Iterating on our input data, 
\begin{equation} \label{eq:skip-connections-3}
\begin{aligned}
    &\begin{bmatrix}
        \Wy{I}     & 0                 & 0      & 0 \\
        \Wg{f_{\theta_1}}   & 0                 & 0      & 0 \\
        0          & \Wg{f_{\theta_2}}          & 0      & 0 \\
        \eta\Wb{S} & 0                 & \Wg{f_{\theta_3}} & 0 \\
    \end{bmatrix}
        \circ
    \begin{bmatrix}
        \Wy{I}      & 0                 & 0        & 0 \\
        \Wg{f_{\theta_1}}    & 0                 & 0        & 0 \\
        0           & \Wg{f_{\theta_2}}          & 0        & 0 \\
        \eta\Wb{S}  & 0                 & \Wg{f_{\theta_3}} & 0 \\
    \end{bmatrix}
        \circ
    \begin{bmatrix}
        \Wy{I}            & 0                 & 0      & 0 \\
        \Wg{f_{\theta_1}} & 0                 & 0      & 0 \\
        0                 & \Wg{f_{\theta_2}} & 0      & 0 \\
        \eta\Wb{S}    & 0                 & \Wg{f_{\theta_3}} & 0 \\
    \end{bmatrix}
        \circ
    \begin{bmatrix}
        \mv{h}_0 \\
        0 \\
        0 \\
        0 \\
    \end{bmatrix}  \\
    &= 
    \begin{bmatrix}
        \mv{h}_0 \\
        \Wg{f_{\theta_1}}(\mv{h}_0) \\
        \Wg{f_{\theta_2}}(\Wg{f_{\theta_1}}(\mv{h}_0)) \\
        \eta \Wb{S(\mv{h}_0)} + \Wg{f_{\theta_3}}(\Wg{f_{\theta_2}}(\Wg{f_{\theta_1}}(\mv{h}_0))) \\
    \end{bmatrix}.
\end{aligned}
\end{equation}
This is also a fixed point since
\begin{equation} \label{eq:skip-connections-4}
    \begin{aligned}
        SK(\eta) \circ 
        \begin{bmatrix}
            \mv{h}_0 \\
            \Wg{f_{\theta_1}}(\mv{h}_0) \\
            \Wg{f_{\theta_2}}(\Wg{f_{\theta_1}}(\mv{h}_0)) \\
            \eta \Wb{S(\mv{h}_0)} + \Wg{f_{\theta_3}}(\Wg{f_{\theta_2}}(\Wg{f_{\theta_1}}(\mv{h}_0))) \\
        \end{bmatrix}=
        \begin{bmatrix}
            \mv{h}_0 \\
            \Wg{f_{\theta_1}}(\mv{h}_0) \\
            \Wg{f_{\theta_2}}(\Wg{f_{\theta_1}}(\mv{h}_0)) \\
            \eta \Wb{S(\mv{h}_0)} + \Wg{f_{\theta_3}}(\Wg{f_{\theta_2}}(\Wg{f_{\theta_1}}(\mv{h}_0))) \\
        \end{bmatrix}
    \end{aligned}
\end{equation}
and is also an infinite impulse response map. Note that as $\eta \rightarrow 0$, this approaches \label{eq:SKIP_Minfty} hence skip connections can be trained via continuation in $\epsilon$ and $\eta$ starting from an MLP!

\subsubsection{Choice of the initial vector}

*** This section is currently blank and I think that is OK. ***

\tblue{The iteration will be independent of the initial vector}
