# Supplementary material for: Rethinking the Relationship between Recurrent and Non-Recurrent Neural Networks: A Study in Sparsity
Source: arXiv:2404.00880 source file (2024-04-01)
Supplement: Supplementary file 6 [file appendix_superdiagonal.tex]

\subsection{Super-diagonal blocks} \label{sec:appendix-superdiagonal}

Now consider
\begin{equation} \label{eq:appendix-superdiagonal-M4}
  M_{ad} = 
    \left[
      \begin{matrix}
  \myI & 0 & 0 & 0\\
  \myfone & 0 & \myS & 0\\
  0 & \myftwo & 0 & 0\\
  0 & 0 & \myfthr & 0
      \end{matrix}
    \right]
  \end{equation}
  
  \begin{equation} \label{eq:appendix-superdiagonal-M4-iteration3}
    \circ_{i=1}^{3}M_{ad}  
      \begin{bmatrix}
          \mv{h}_0 \\
          0 \\
          0 \\
          0 \\
      \end{bmatrix}
     = 
    \begin{bmatrix}
  \mv{h}_0 \\
  \myfone \circ \mv{h}_0 + \myS \circ \myftwo \circ \myfone \circ \mv{h}_0 \\
  \myftwo \circ \myfone \circ \mv{h}_0 \\
  \myfthr \circ \myftwo \circ \myfone \circ \mv{h}_0 
      \end{bmatrix}
  \end{equation}
  
  \begin{equation} \label{eq:appendix-superdiagonal-M4-iteration4}
    \circ_{i=1}^{4}M_{ad}  
      \begin{bmatrix}
          \mv{h}_0 \\
          0 \\
          0 \\
          0 \\
      \end{bmatrix}
     = 
      \begin{bmatrix}
  \mv{h}_0 \\
  \myfone \circ \mv{h}_0 + \myS \circ \myftwo \circ \myfone \circ \mv{h}_0   \\
  \myftwo \circ \myfone \circ \mv{h}_0 + \myftwo \circ \myS \circ \myftwo \circ \myfone \circ \mv{h}_0   \\
  \myfthr \circ \myftwo \circ \myfone \circ \mv{h}_0 
      \end{bmatrix}
  \end{equation}
  
  \begin{equation} \label{eq:appendix-superdiagonal-M4-iteration5}
    \circ_{i=1}^{5}M_{ad}  
      \begin{bmatrix}
          \mv{h}_0 \\
          0 \\
          0 \\
          0 \\
      \end{bmatrix}
 = 
      \begin{bmatrix}
  \mv{h}_0 \\
  \myfone \circ \mv{h}_0 +  \myS \circ \myftwo \circ \myfone \circ \mv{h}_0 + \myS \circ \myftwo \circ \myS \circ \myftwo \circ \myfone \circ \mv{h}_0    \\
  \myftwo \circ \myfone \circ \mv{h}_0 + \myftwo \circ \myS \circ \myftwo \circ \myfone \circ \mv{h}_0   \\
  \myfthr \circ \myftwo \circ \myfone \circ \mv{h}_0 + \myfthr \circ \myftwo \circ \myS \circ \myftwo \circ \myfone \circ \mv{h}_0  
      \end{bmatrix}
  \end{equation}
  
  In general, after the $k$-th iteration, if $S$ and $f_{\theta_i}$ are linear, with $k$ odd and $k \ge 3$ we have

  \begin{equation} \label{eq:appendix-superdiagonal-M4-iterationk-odd}
    \circ_{i=1}^{k} M_{ad}  
      \begin{bmatrix}
          \mv{h}_0 \\
          0 \\
          0 \\
          0 \\
      \end{bmatrix}
   = 
      \begin{bmatrix}
  \mv{h}_0 \\
  ( \circ_{i=0}^{\frac{k-1}{2}} (\myS \circ \myftwo) ) \circ \myfone \circ \mv{h}_0 \\
  \myftwo \circ ( \circ_{i=0}^{\frac{k-3}{2}} (\myS \circ \myftwo) ) \circ \myfone \circ \mv{h}_0 \\
  \myfthr \circ \myftwo \circ ( \circ_{i=0}^{\frac{k-3}{2}} (\myS \circ \myftwo) ) \circ \myfone \circ \mv{h}_0 
      \end{bmatrix}
  \end{equation}

After the $k$-th iteration, if $S$ and $f_{\theta_i}$ are linear, with $k$ even and $k \ge 4$ we have

  \begin{equation} \label{eq:appendix-superdiagonal-M4-iterationk-even}
    \circ_{i=1}^{k} M_{ad}  
      \begin{bmatrix}
          \mv{h}_0 \\
          0 \\
          0 \\
          0 \\
      \end{bmatrix}
= 
      \begin{bmatrix}
  \mv{h}_0 \\
  ( \circ_{i=0}^{\frac{k-3}{2}} (\myS \circ \myftwo) ) \circ \myfone \circ \mv{h}_0 \\
  \myftwo \circ ( \circ_{i=0}^{\frac{k-3}{2}} (\myS \circ \myftwo) ) \circ \myfone \circ \mv{h}_0 \\
  \myfthr \circ \myftwo \circ ( \circ_{i=0}^{\frac{k-4}{2}} (\myS \circ \myftwo) ) \circ \myfone \circ \mv{h}_0 
      \end{bmatrix}
  \end{equation}

So, in the liner case, the convergence of the above is determined by the convergence of the infinite product of $S \circ \myftwo$ alone!  Note, here $\myftwo$, and the $f_{\theta_j}$, are generally non-linear functions and the power-series is not available in closed form.  However, perhaps special cases of $f_{\theta_j}$ can be considered.

% \subsection{Top row of zeros} \label{sec:generalizations-RNN}

% Assigning zero blocks to the top row recalls the RNN \eqref{eq:RNN-dyamics}, i.e, 
% % Full matrix
% \begin{equation} \label{eq:generalizations-RNN}
%     \begin{bmatrix}
%         0 & 0  & 0  & 0  & 0 \\
%         \Wg{W_{2,1}} & \Wy{W_{2,2}}  & \Wr{W_{2,3}}  & \Wr{W_{2,4}}  & \Wr{W_{2,5}} \\
%         \Wb{W_{3,1}} & \Wg{W_{3,2}}  & \Wy{W_{3,3}}  & \Wr{W_{3,4}}  & \Wr{W_{3,5}} \\
%         \Wb{W_{4,1}} & \Wb{W_{4,2}}  & \Wg{W_{4,3}}  & \Wy{W_{4,4}}  & \Wr{W_{4,5}} \\
%         \Wb{W_{5,1}} & \Wb{W_{5,2}}  & \Wb{W_{5,3}}  & \Wg{W_{5,4}}  & \Wy{W_{5,5}} \\
%     \end{bmatrix}
%     =
%     \begin{bmatrix}
%         0 & 0 \\
%         W_1 & W_2 \\
%     \end{bmatrix}
% \end{equation}
% which is an RNN.

\subsubsection{\tblue{Choice of the initial vector}}\label{sec:appendix-superdiagonal-q}

\tblue{The iteration will {\bf not} be independent of the initial vector.} Note that after three iterations
\begin{equation} \label{eq:appendix-superdiagonal-iteration3q}
    \circ_{i=1}^{3}M_{ad}  
      \begin{bmatrix}
          \mv{h}_0 \\
          q_1 \\
          q_2 \\
          q_3 \\
      \end{bmatrix}
 = 
      \begin{bmatrix}
  \mv{h}_0 \\
  \myfone \circ \mv{h}_0 + \myS \circ \myftwo \circ \myfone \circ \mv{h}_0 + \myS \circ \myftwo \circ \myS \circ q_2 ) \\
  \myftwo \circ \myfone \circ \mv{h}_0 + \myftwo \circ \myS \circ \myftwo \circ q_1 \\
  \myfthr \circ \myftwo \circ \myfone \circ \mv{h}_0  + \myfthr \circ \myftwo \circ \myS \circ q_2
      \end{bmatrix}
  \end{equation}
