# Supplementary material for: Rethinking the Relationship between Recurrent and Non-Recurrent Neural Networks: A Study in Sparsity
Source: arXiv:2404.00880 source file (2024-04-01)
Supplement: Supplementary file 7 [file Additional_iterations.tex]

\section{Additional Iterations} \label{sec:additional-iterations}

\subsection{RNN with additional iterations}\label{sec:RNN-additional-iterations}
\subsubsection{Finite impulse response}

%In \S \ref{sec:RNN-block-iterative} it is important to recognize that the \eqref{eq:RNN-iterative-matrix-T} starting with initial conditions \eqref{eq:RNN-iterative-initial-condition-T} must be iterated $T$ times to achieve the equivalent outcome as \eqref{eq:RNN-defn}. Further iterations lead to undesirable results as shown below.

Applying the map $M_{RNN}$ one additional time reveals 
\begin{equation} \label{eq:RNN-iteration-4}
\begin{aligned}
    M \circ 
    M \circ 
    M \circ 
    M \circ 
    \begin{bmatrix}
        \mv{h}_0 \\
        0 \\
        0 \\
        0 \\
    \end{bmatrix} 
    &=       
    \begin{bmatrix}
        0                             & 0                             & 0                             & 0 \\
        \Wg{f_\theta(\cdot,\mv{x}_1)} & 0                             & 0                             & 0 \\
        0                             & \Wg{f_\theta(\cdot,\mv{x}_2)} & 0                             & 0 \\
        0                             & 0                             & \Wg{f_\theta(\cdot,\mv{x}_3)} & 0 \\
    \end{bmatrix}
    \circ 
    \begin{bmatrix}
        0 \\
        \Wg{f_\theta(0,\mv{x}_1)} \\
        \Wg{f_\theta \big( f_\theta(0,\mv{x}_1) ,\mv{x}_2 \big)} \\
        \Wg{f_\theta \Big(  f_\theta \big( f_\theta(\mv{h}_0,\mv{x}_1),\mv{x}_2 \big),\mv{x}_3} \Big)  \\
    \end{bmatrix} \\
    &=
    \begin{bmatrix}
        0 \\
        \Wg{f_\theta(0,\mv{x}_1)} \\
        \Wg{f_\theta \big( f_\theta(0,\mv{x}_1) ,\mv{x}_2 \big)} \\
        \Wg{f_\theta \Big(  f_\theta \big( f_\theta(0,\mv{x}_1),\mv{x}_2 \big),\mv{x}_3} \Big)  \\
    \end{bmatrix}
\end{aligned}
\end{equation}
which is independent of the input $\mv{h}_0$.

\subsubsection{Fixed point} \label{sec:RNN-fixed-point}
An additional application of $M_{RNN}$ 
\begin{equation} \label{eq:RNN_fixed_point}
\begin{aligned}
    M \circ 
    M \circ 
    M \circ 
    M \circ 
    M \circ
    \begin{bmatrix}
        \mv{h}_0 \\
        0 \\
        0 \\
        0 \\
    \end{bmatrix} 
    &=
    \begin{bmatrix}
        0                             & 0                             & 0                             & 0 \\
        \Wg{f_\theta(\cdot,\mv{x}_1)} & 0                             & 0                             & 0 \\
        0                             & \Wg{f_\theta(\cdot,\mv{x}_2)} & 0                             & 0 \\
        0                             & 0                             & \Wg{f_\theta(\cdot,\mv{x}_3)} & 0 \\
    \end{bmatrix}
    \circ 
    \begin{bmatrix}
        0 \\
        \Wg{f_\theta(0,\mv{x}_1)} \\
        \Wg{f_\theta \big( f_\theta(0,\mv{x}_1) ,\mv{x}_2 \big)} \\
        \Wg{f_\theta \Big(  f_\theta \big( f_\theta(0,\mv{x}_1),\mv{x}_2 \big),\mv{x}_3} \Big)  \\
    \end{bmatrix} \\ 
    &=
 \begin{bmatrix}
        0 \\
        \Wg{f_\theta(0,\mv{x}_1)} \\
        \Wg{f_\theta \big( f_\theta(0,\mv{x}_1) ,\mv{x}_2 \big)} \\
        \Wg{f_\theta \Big(  f_\theta \big( f_\theta(0,\mv{x}_1),\mv{x}_2 \big),\mv{x}_3} \Big)  \\
    \end{bmatrix}
\end{aligned}
\end{equation}
which in addition, shows that 
\begin{equation} \label{eq:MLP_fixed_point}
\begin{bmatrix}
        0 \\
        \Wg{f_\theta(0,\mv{x}_1)} \\
        \Wg{f_\theta \big( f_\theta(0,\mv{x}_1) ,\mv{x}_2 \big)} \\
        \Wg{f_\theta \Big(  f_\theta \big( f_\theta(0,\mv{x}_1),\mv{x}_2 \big),\mv{x}_3} \Big)  \\
    \end{bmatrix}  
\end{equation}
is a fixed point.
