# Supplementary material for: Rethinking the Relationship between Recurrent and Non-Recurrent Neural Networks: A Study in Sparsity
Source: arXiv:2404.00880 source file (2024-04-01)
Supplement: Supplementary file 8 [file appendix.tex]

\renewcommand\Wr[1]{\colorbox{red}{$#1$}}
\renewcommand\Wg[1]{\colorbox{green}{$#1$}}
\renewcommand\Wb[1]{\colorbox{blue}{$#1$}}
\renewcommand\Wy[1]{\colorbox{yellow}{$#1$}}

\section{Arbitrarily close to finite impulse response maps}
\todo{Randy will take this first pass to revising the appendices}
Now consider 
\begin{equation} \label{eq:nearby-maps-Minfty-epsilon}
    M_{\infty}(\epsilon) =
    \begin{bmatrix}
        \epsilon \Wy{I}   & 0                 & 0                 & 0 \\
        \Wg{f_{\theta_1}}          & 0                 & 0                 & 0 \\
        0                 & \Wg{f_{\theta_2}}          & 0                 & 0 \\
        0                 & 0                 & \Wg{f_{\theta_3}}          & 0 \\
    \end{bmatrix}.
\end{equation}
where $0 \le \epsilon \le 1$ which as $\epsilon \rightarrow 0$ becomes arbitrarily close to a finite impulse response map.  In fact, it is exactly an finite impulse response map when $\epsilon=0$ and an infinite impulse response map when $\epsilon=1$. Defining
\begin{equation} \label{eq:SKIP_Minfty_epsilon_k}
    \circ_{i=1}^k M_{\infty}(\epsilon) = M_{\infty}(\epsilon) \circ M_{\infty}(\epsilon) \circ \dots \circ M_{\infty}(\epsilon) 
\end{equation}
for any value of $\epsilon$ after three iterations, 
\begin{equation} \label{eq:nearby-maps-Minfty-epsilon-3}
    \circ_{i=1}^3 M_{\infty}(\epsilon) = 
    M_{\infty}(\epsilon) \circ 
    M_{\infty}(\epsilon) \circ 
    M_{\infty}(\epsilon) \circ 
    \begin{bmatrix}
        \mv{h}_0 \\
        0 \\
        0 \\
        0 \\
    \end{bmatrix} 
    = \begin{bmatrix}
        \epsilon^3 \mv{h}_0 \\
        \Wg{f_{\theta_1}}(\epsilon^2 \mv{h}_0) \\
        \Wg{f_{\theta_2}}(\Wg{f_{\theta_1}}(\epsilon \mv{h}_0)) \\
        \Wg{f_{\theta_3}}(\Wg{f_{\theta_2}}(\Wg{f_{\theta_1}}(\mv{h}_0)))  \\
    \end{bmatrix}
\end{equation}.
After four iterations,
\begin{equation} \label{eq:nearby-maps-Minfty-epsilon-4}
    \circ_{i=1}^4 M_{\infty}(\epsilon) =
    M_{\infty}(\epsilon) \circ 
    M_{\infty}(\epsilon) \circ 
    M_{\infty}(\epsilon) \circ 
    M_{\infty}(\epsilon) \circ 
    \begin{bmatrix}
        \mv{h}_0 \\
        0 \\
        0 \\
        0 \\
    \end{bmatrix} 
    = \begin{bmatrix}
        \epsilon^4 \mv{h}_0 \\
        \Wg{f_{\theta_1}}(\epsilon^3 \mv{h}_0) \\
        \Wg{f_{\theta_2}}(\Wg{f_{\theta_1}}(\epsilon^2 \mv{h}_0)) \\
        \Wg{f_{\theta_3}}(\Wg{f_{\theta_2}}(\Wg{f_{\theta_1}}(\epsilon \mv{h}_0)))  \\
    \end{bmatrix}
\end{equation}
Further,
\begin{equation} \label{eq:nearby-maps-Minfty-epsilon-k}
    \circ_{i=1}^k M_{\infty}(\epsilon) 
    \left(
    \begin{bmatrix}
        \mv{h}_0 \\
        0 \\
        0 \\
        0 \\
    \end{bmatrix}
    \right) 
    = \begin{bmatrix}
        \epsilon^k \mv{h}_0 \\
        \Wg{f_{\theta_1}}(\epsilon^{k-1} \mv{h}_0) \\
        \Wg{f_{\theta_2}}(\Wg{f_{\theta_1}}(\epsilon^{k-2} \mv{h}_0)) \\
        \Wg{f_{\theta_3}}(\Wg{f_{\theta_2}}(\Wg{f_{\theta_1}}(\epsilon^{k-3} \mv{h}_0)))  \\
    \end{bmatrix}
\end{equation}
hence if it \emph{converges} to a finite impulse map when $\epsilon \rightarrow 0$ and $f_{\theta_i}=0, \forall i=1, 2, 3$. Further, for $0 < \epsilon < 1$ converges \emph{asymptotically} to a finite impulse map as $k \rightarrow \infty$ and $f_{\theta_i}=0, \forall i=1, \dots, k$. We conclude there is a \emph{continuum}, parametrized by $\epsilon$ between a finite impulse response map, and a response map whose impulse response approaches zero \emph{asymptotically}, and a recurrent neural network with infinite (non-converging) impulse response.

\subsection{Skip Connections} \label{sec:skip-connections}

Define
\begin{equation} \label{eq:nearby-maps-skip}
    SK(\eta)=
    \begin{bmatrix}
        \Wy{I}        & 0                 & 0        & 0 \\
        \Wg{f_1}      & 0                 & 0        & 0 \\
        0             & \Wg{f_2}          & 0        & 0 \\
        \eta\Wb{S}    & 0                 & \Wg{f_3} & 0 \\
    \end{bmatrix}.
\end{equation}
Iterating on our input data , 
\begin{equation} \label{eq:nearby-maps-skip-3}
\begin{aligned}
    &\begin{bmatrix}
        \Wy{I}     & 0                 & 0      & 0 \\
        \Wg{f_1}   & 0                 & 0      & 0 \\
        0          & \Wg{f_2}          & 0      & 0 \\
        \eta\Wb{S} & 0                 & \Wg{f_3} & 0 \\
    \end{bmatrix}
        \circ
    \begin{bmatrix}
        \Wy{I}      & 0                 & 0        & 0 \\
        \Wg{f_1}    & 0                 & 0        & 0 \\
        0           & \Wg{f_2}          & 0        & 0 \\
        \eta\Wb{S}  & 0                 & \Wg{f_3} & 0 \\
    \end{bmatrix}
        \circ
    \begin{bmatrix}
        \Wy{I}            & 0                 & 0      & 0 \\
        \Wg{f_1} & 0                 & 0      & 0 \\
        0                 & \Wg{f_2} & 0      & 0 \\
        \eta\Wb{S}    & 0                 & \Wg{f_3} & 0 \\
    \end{bmatrix}
        \circ
    \begin{bmatrix}
        \mv{h}_0 \\
        0 \\
        0 \\
        0 \\
    \end{bmatrix}  \\
    &= 
    \begin{bmatrix}
        \mv{h}_0 \\
        \Wg{f_1}(\mv{h}_0) \\
        \Wg{f_2}(\Wg{f_1}(\mv{h}_0)) \\
        \eta \Wb{S(\mv{h}_0)} + \Wg{f_3}(\Wg{f_2}(\Wg{f_1}(\mv{h}_0))) \\
    \end{bmatrix}.
\end{aligned}
\end{equation}
This is also a fixed point since
\begin{equation} \label{eq:nearby-maps-skip-4}
    \begin{aligned}
        SK(\eta) \circ 
        \begin{bmatrix}
            \mv{h}_0 \\
            \Wg{f_1}(\mv{h}_0) \\
            \Wg{f_2}(\Wg{f_1}(\mv{h}_0)) \\
            \eta \Wb{S(\mv{h}_0)} + \Wg{f_3}(\Wg{f_2}(\Wg{f_1}(\mv{h}_0))) \\
        \end{bmatrix}=
        \begin{bmatrix}
            \mv{h}_0 \\
            \Wg{f_1}(\mv{h}_0) \\
            \Wg{f_2}(\Wg{f_1}(\mv{h}_0)) \\
            \eta \Wb{S(\mv{h}_0)} + \Wg{f_3}(\Wg{f_2}(\Wg{f_1}(\mv{h}_0))) \\
        \end{bmatrix}
    \end{aligned}
\end{equation}
and is also an infinite impulse response map. Note that as $\eta \rightarrow 0$, this approaches \label{eq:SKIP_Minfty} hence skip connections can be trained via continuation in $\epsilon$ and $\eta$ starting from an MLP!  

% \begin{equation}
%     C(0) 
%     \circ 
%     C(0)
%     \circ
%     C(0) \circ Y
%     =\begin{bmatrix}
%          X \\
%         f_{\theta_1}(X) \\
%         f_{\theta_2}(f_{\theta_1}(X)) \\
%         f_{\theta_3}(f_{\theta_2}(f_{\theta_1}(X))) \\
%       \end{bmatrix} 
% \end{equation}
% which is a fixed point and therefore has infinite impulse response. We conclude that $C(0)$ is an CNN. Note that 
% \begin{equation}
%     C(\epsilon) \circ Z(\epsilon)
%     = \begin{bmatrix}
%         (1-\epsilon)^4 X \\
%         (1-\epsilon)^3 f_{\theta_1}(X) \\
%         (1-\epsilon)^2 f_{\theta_2}(f_{\theta_1}(X)) \\
%         (1-\epsilon)^4 S(X) + (1-\epsilon) f_{\theta_3}(f_{\theta_2}(f_{\theta_1}(X))) \\
%       \end{bmatrix} 
%       \rightarrow 
%       \begin{bmatrix}
%         0 \\
%         0 \\
%         0 \\
%         0 \\
%       \end{bmatrix} 
%       \; \hbox{as} \; \epsilon \rightarrow 1.
% \end{equation}

% \subsection{MultilLayer Perceptrons}
% Note that $C(1)=B$ and when $X=[x_0, x_0, \dots, x_0]$, \todo{This is not what a minibatch means here I think}

% i.e., the columns of $X$ are simply replicates of the initial data, then 
% \begin{equation}
%     C(1) \circ C(1) \circ C(1) \circ Y
% \end{equation}
% is a multilayer perceptron with finite impulse response. Similarly we can define MLPs
% \begin{equation}
%     C(\epsilon) \circ C(\epsilon) \circ C(\epsilon) \circ Y \quad  0 \le \epsilon < 1
% \end{equation}
% with infinite impulse response. We conclude that when viewed in this block iterative framework, there is no difference between a SNN or RNN and a MLP with finite or infinite impulse response, but the data contained within the matrix $X$. 
