# Supplementary material for: Rethinking the Relationship between Recurrent and Non-Recurrent Neural Networks: A Study in Sparsity
Source: arXiv:2404.00880 source file (2024-04-01)
Supplement: Supplementary file 9 [file appendixv2.tex]

\renewcommand\Wr[1]{\colorbox{red}{$#1$}}
\renewcommand\Wg[1]{\colorbox{green}{$#1$}}
\renewcommand\Wb[1]{\colorbox{blue}{$#1$}}
\renewcommand\Wy[1]{\colorbox{yellow}{$#1$}}

\section{Generalizations} 
\label{sec:generalizations}

\subsection{TBD} \label{sec:sequential2D}
\todo{This section needs to be cleaned up.  There are twp versions of the same thing.  Use the colored one, but keep the points from the earlier one.}
% \begin{definition} \label{defn:seqential2D}
% Sequential2D is a rectangular block matrix function within which each entry is a matrix function. A Sequential2D map is of the form
% \begin{equation} \label{eq:Sequential2D}
%     M = \begin{bmatrix} D_{11} &A_{12}  &\hdots &A_{1n}  \\
%                         A_{21} &D_{22} &\hdots &A_{2n}  \\
%                         \vdots &       &\ddots &\vdots \\
%                         A_{n1} &A_{n2} &\hdots &D_{nn}
%         \end{bmatrix}                    
% \end{equation}
% where at least one of $A_{ij}, i \not= j$ is non-zero.
% By contrast Sequential1D maps are a subset of Sequential2D maps of the form
% \begin{equation} \label{eq:Sequential1D}
%     M = \begin{bmatrix} D_{11} &0      &\hdots  &0  \\
%                         D_{22} &0      &\hdots  &0  \\
%                         \vdots &\vdots &\ddots  &\vdots \\
%                         D_{nn} &0      &\hdots  &0
%         \end{bmatrix}                    
% \end{equation}

% \end{definition}
% In many ways, \eqref{eq:Sequential2D} is a straightforward generalization of a block-defined matrix.  In particular, if every function $A_{ij}$ happened to be linear (i.e., a matrix) and the function composition operator $\circ$ were replaced with the dot-product, then \eqref{eq:Sequential2D} would be precisely a block defined matrix. 

TBD TBD TBD TBD TBD TBD TBD TBD
TBD TBD TBD TBD TBD TBD TBD TBD
TBD TBD TBD TBD TBD TBD TBD TBD
TBD TBD TBD TBD TBD TBD TBD TBD
TBD TBD TBD TBD TBD TBD TBD TBD
TBD TBD TBD TBD TBD TBD TBD TBD
TBD TBD TBD TBD TBD TBD TBD TBD
TBD TBD TBD TBD TBD TBD TBD TBD
TBD TBD TBD TBD TBD TBD TBD TBD
TBD TBD TBD TBD TBD TBD TBD TBD
TBD TBD TBD TBD TBD TBD TBD TBD
TBD TBD TBD TBD TBD TBD TBD TBD
This opens an entire range of new possibilities when considering a block iterative function of the form

% Full matrix
\begin{equation} \label{eq:generalizations-full}
    \begin{bmatrix}
        \Wy{W_{1,1}} & \Wr{W_{1,2}}  & \Wr{W_{1,3}}  & \Wr{W_{1,4}}  & \Wr{W_{1,5}} \\
        \Wg{W_{2,1}} & \Wy{W_{2,2}}  & \Wr{W_{2,3}}  & \Wr{W_{2,4}}  & \Wr{W_{2,5}} \\
        \Wb{W_{3,1}} & \Wg{W_{3,2}}  & \Wy{W_{3,3}}  & \Wr{W_{3,4}}  & \Wr{W_{3,5}} \\
        \Wb{W_{4,1}} & \Wb{W_{4,2}}  & \Wg{W_{4,3}}  & \Wy{W_{4,4}}  & \Wr{W_{4,5}} \\
        \Wb{W_{5,1}} & \Wb{W_{5,2}}  & \Wb{W_{5,3}}  & \Wg{W_{5,4}}  & \Wy{W_{5,5}} \\
    \end{bmatrix}
\end{equation}

In this notation, 
\begin{itemize}
\item $\Wr{W_{i-k,i}}, \; k>1$ corresponds to TBD TBD TBD TBD TBD TBD TBD TBD TBD TBD TBD TBD TBD TBD TBD.
\item $\Wy{W_{i,i}}$ corresponds to TBD TBD TBD TBD TBD TBD TBD TBD TBD TBD TBD TBD TBD TBD TBD.
\item $\Wg{W_{i+1,i}}$ corresponds to a standard MLP or, more generally, an NN that can be implemented as a Pytorch or Keras Sequential container.
\item $\Wb{W_{i+k,i}}, \; k>1$ corresponds to skip connections and finite impulse response (FIR) filters.
%\item We began the exploration of $\Wy{W_{i,i}}$ with the introduction of the $I$ in \eqref{FIXME} corresponds infinite impulse response filters.
%\item What do $\Wr{W_{i,j}}, \; j>i$ correspond to?  They are actually \emph{feedback} connections which also lead to infinite impulse response filters and classic RNNs.
\end{itemize}

\subsection{Arbitrarily close to finite impulse response maps}
Now consider 
\begin{equation} \label{eq:nearby-maps-Minfty-epsilon}
    M_{\infty}(\epsilon) =
    \begin{bmatrix}
        \epsilon \Wy{I}   & 0                 & 0                 & 0 \\
        \Wg{f_{\theta_1}}          & 0                 & 0                 & 0 \\
        0                 & \Wg{f_{\theta_2}}          & 0                 & 0 \\
        0                 & 0                 & \Wg{f_{\theta_3}}          & 0 \\
    \end{bmatrix}.
\end{equation}
where $0 \le \epsilon \le 1$ which as $\epsilon \rightarrow 0$ becomes arbitrarily close to a finite impulse response map.  In fact, it is exactly an finite impulse response map when $\epsilon=0$ and an infinite impulse response map when $\epsilon=1$. Defining
\begin{equation} \label{eq:SKIP_Minfty_epsilon_k}
    \circ_{i=1}^k M_{\infty}(\epsilon) = M_{\infty}(\epsilon) \circ M_{\infty}(\epsilon) \circ \dots \circ M_{\infty}(\epsilon) 
\end{equation}
for any value of $\epsilon$ after three iterations, 
\begin{equation} \label{eq:nearby-maps-Minfty-epsilon-3}
    \circ_{i=1}^3 M_{\infty}(\epsilon) = 
    M_{\infty}(\epsilon) \circ 
    M_{\infty}(\epsilon) \circ 
    M_{\infty}(\epsilon) \circ 
    \begin{bmatrix}
        \mv{h}_0 \\
        0 \\
        0 \\
        0 \\
    \end{bmatrix} 
    = \begin{bmatrix}
        \epsilon^3 \mv{h}_0 \\
        \Wg{f_{\theta_1}}(\epsilon^2 \mv{h}_0) \\
        \Wg{f_{\theta_2}}(\Wg{f_{\theta_1}}(\epsilon \mv{h}_0)) \\
        \Wg{f_{\theta_3}}(\Wg{f_{\theta_2}}(\Wg{f_{\theta_1}}(\mv{h}_0)))  \\
    \end{bmatrix}
\end{equation}.
After four iterations,
\begin{equation} \label{eq:nearby-maps-Minfty-epsilon-4}
    \circ_{i=1}^4 M_{\infty}(\epsilon) =
    M_{\infty}(\epsilon) \circ 
    M_{\infty}(\epsilon) \circ 
    M_{\infty}(\epsilon) \circ 
    M_{\infty}(\epsilon) \circ 
    \begin{bmatrix}
        \mv{h}_0 \\
        0 \\
        0 \\
        0 \\
    \end{bmatrix} 
    = \begin{bmatrix}
        \epsilon^4 \mv{h}_0 \\
        \Wg{f_{\theta_1}}(\epsilon^3 \mv{h}_0) \\
        \Wg{f_{\theta_2}}(\Wg{f_{\theta_1}}(\epsilon^2 \mv{h}_0)) \\
        \Wg{f_{\theta_3}}(\Wg{f_{\theta_2}}(\Wg{f_{\theta_1}}(\epsilon \mv{h}_0)))  \\
    \end{bmatrix}
\end{equation}
Further,
\begin{equation} \label{eq:nearby-maps-Minfty-epsilon-k}
    \circ_{i=1}^k M_{\infty}(\epsilon) 
    \left(
    \begin{bmatrix}
        \mv{h}_0 \\
        0 \\
        0 \\
        0 \\
    \end{bmatrix}
    \right) 
    = \begin{bmatrix}
        \epsilon^k \mv{h}_0 \\
        \Wg{f_{\theta_1}}(\epsilon^{k-1} \mv{h}_0) \\
        \Wg{f_{\theta_2}}(\Wg{f_{\theta_1}}(\epsilon^{k-2} \mv{h}_0)) \\
        \Wg{f_{\theta_3}}(\Wg{f_{\theta_2}}(\Wg{f_{\theta_1}}(\epsilon^{k-3} \mv{h}_0)))  \\
    \end{bmatrix}
\end{equation}
hence if it \emph{converges} to a finite impulse map when $\epsilon \rightarrow 0$ and $f_{\theta_i}=0, \forall i=1, 2, 3$. Further, for $0 < \epsilon < 1$ converges \emph{asymptotically} to a finite impulse map as $k \rightarrow \infty$ and $f_{\theta_i}=0, \forall i=1, \dots, k$. We conclude there is a \emph{continuum}, parametrized by $\epsilon$ between a finite impulse response map, and a response map whose impulse response approaches zero \emph{asymptotically}, and a recurrent neural network with infinite (non-converging) impulse response.

\subsection{Skip Connections} \label{sec:skip-connections}

Define
\begin{equation} \label{eq:nearby-maps-skip}
    SK(\eta)=
    \begin{bmatrix}
        \Wy{I}        & 0                 & 0        & 0 \\
        \Wg{f_{\theta_1}}      & 0                 & 0        & 0 \\
        0             & \Wg{f_{\theta_2}}          & 0        & 0 \\
        \eta\Wb{S}    & 0                 & \Wg{f_{\theta_3}} & 0 \\
    \end{bmatrix}.
\end{equation}
Iterating on our input data , 
\begin{equation} \label{eq:nearby-maps-skip-3}
\begin{aligned}
    &\begin{bmatrix}
        \Wy{I}     & 0                 & 0      & 0 \\
        \Wg{f_{\theta_1}}   & 0                 & 0      & 0 \\
        0          & \Wg{f_{\theta_2}}          & 0      & 0 \\
        \eta\Wb{S} & 0                 & \Wg{f_{\theta_3}} & 0 \\
    \end{bmatrix}
        \circ
    \begin{bmatrix}
        \Wy{I}      & 0                 & 0        & 0 \\
        \Wg{f_{\theta_1}}    & 0                 & 0        & 0 \\
        0           & \Wg{f_{\theta_2}}          & 0        & 0 \\
        \eta\Wb{S}  & 0                 & \Wg{f_{\theta_3}} & 0 \\
    \end{bmatrix}
        \circ
    \begin{bmatrix}
        \Wy{I}            & 0                 & 0      & 0 \\
        \Wg{f_{\theta_1}} & 0                 & 0      & 0 \\
        0                 & \Wg{f_{\theta_2}} & 0      & 0 \\
        \eta\Wb{S}    & 0                 & \Wg{f_{\theta_3}} & 0 \\
    \end{bmatrix}
        \circ
    \begin{bmatrix}
        \mv{h}_0 \\
        0 \\
        0 \\
        0 \\
    \end{bmatrix}  \\
    &= 
    \begin{bmatrix}
        \mv{h}_0 \\
        \Wg{f_{\theta_1}}(\mv{h}_0) \\
        \Wg{f_{\theta_2}}(\Wg{f_{\theta_1}}(\mv{h}_0)) \\
        \eta \Wb{S(\mv{h}_0)} + \Wg{f_{\theta_3}}(\Wg{f_{\theta_2}}(\Wg{f_{\theta_1}}(\mv{h}_0))) \\
    \end{bmatrix}.
\end{aligned}
\end{equation}
This is also a fixed point since
\begin{equation} \label{eq:nearby-maps-skip-4}
    \begin{aligned}
        SK(\eta) \circ 
        \begin{bmatrix}
            \mv{h}_0 \\
            \Wg{f_{\theta_1}}(\mv{h}_0) \\
            \Wg{f_{\theta_2}}(\Wg{f_{\theta_1}}(\mv{h}_0)) \\
            \eta \Wb{S(\mv{h}_0)} + \Wg{f_{\theta_3}}(\Wg{f_{\theta_2}}(\Wg{f_{\theta_1}}(\mv{h}_0))) \\
        \end{bmatrix}=
        \begin{bmatrix}
            \mv{h}_0 \\
            \Wg{f_{\theta_1}}(\mv{h}_0) \\
            \Wg{f_{\theta_2}}(\Wg{f_{\theta_1}}(\mv{h}_0)) \\
            \eta \Wb{S(\mv{h}_0)} + \Wg{f_{\theta_3}}(\Wg{f_{\theta_2}}(\Wg{f_{\theta_1}}(\mv{h}_0))) \\
        \end{bmatrix}
    \end{aligned}
\end{equation}
and is also an infinite impulse response map. Note that as $\eta \rightarrow 0$, this approaches \label{eq:SKIP_Minfty} hence skip connections can be trained via continuation in $\epsilon$ and $\eta$ starting from an MLP!  


\subsection{Diagonal blocks} \label{sec:generalizations-diagonal}

Let
\begin{equation}\label{eq:generalizations-diagonal}
M_{d4} = 
  \left[
      \begin{matrix}
  \Wy{I} & 0 & 0 & 0\\
  \myfone & \Wy{S} & 0 & 0\\
  0 & \myftwo & 0 & 0\\
  0 & 0 & \myfthr & 0
      \end{matrix}
    \right]
  \end{equation}

Note that after three iterations
  \begin{equation} \label{eq:generalizations-diagonal-M3-iteration3}
    \circ_{i=1}^3 M_{d}  
    \left(
      \begin{bmatrix}
          \mv{h}_0 \\
          0 \\
          0 \\
          0 \\
      \end{bmatrix}
      \right) = 
    \left[
      \begin{matrix}
  \mv{h}_0 \\
  \myfone \circ \mv{h}_0 + \Wy{S} \circ \myfone \circ \mv{h}_0 +  \Wy{S} \circ \Wy{S} \circ \myfone \circ \mv{h}_0 \\
  \myftwo \circ \myfone \circ \mv{h}_0 + \myftwo \circ \Wy{S} \circ \myfone \circ \mv{h}_0 \\
  \myfthr \circ \myftwo \circ \myfone \circ \mv{h}_0 
      \end{matrix}
    \right]
  \end{equation}

\subsubsection{\tblue{Choice of the initial vector}}

\tblue{The iteration will {\bf not} be independent of the initial vector}

Note that after three iterations
  \begin{equation} \label{eq:generalizations-diagonal-M3-iteration3}
    \circ_{i=1}^3 M_{d}  
    \left(
      \begin{bmatrix}
          \mv{h}_0 \\
          q_1 \\
          q_2 \\
          q_3 \\
      \end{bmatrix}
      \right) = 
    \left[
      \begin{matrix}
  \mv{h}_0 \\
  \myfone \circ \mv{h}_0  + \Wy{S} \circ \myfone \circ \mv{h}_0 +  \Wy{S} \circ \Wy{S} \circ \myfone \circ \mv{h}_0 + \Wy{S} \circ \Wy{S} \circ \Wy{S} \circ q_1  \\
  \myftwo \circ \myfone \circ \mv{h}_0  + \myftwo \circ \Wy{S} \circ \myfone \circ \mv{h}_0 +  \myftwo \circ \Wy{S} \circ \Wy{S} \circ q_1 \\
  \myfthr \circ \myftwo \circ \myfone \circ \mv{h}_0 + \myfthr \circ \myftwo \circ \Wy{S} \circ q_1 
      \end{matrix}
    \right]
  \end{equation}

  
After four iterations
  \begin{equation} \label{eq:generalizations-diagonal-M3-iteration4}
    \circ_{i=1}^4 M_{d}  
    \left(
      \begin{bmatrix}
         \mv{h}_0 \\
          0 \\
          0 \\
          0 \\
      \end{bmatrix}
      \right) = 
    \left[
      \begin{matrix}
  \mv{h}_0 \\
  \Wy{S} \circ \myfone \circ \mv{h}_0 +  \Wy{S} \circ \Wy{S} \circ \myfone \circ \mv{h}_0 +  \Wy{S} \circ \Wy{S} \circ \Wy{S} \circ \myfone \circ \mv{h}_0 +  \myfone \circ \mv{h}_0 \\
  \myftwo \circ \Wy{S} \circ \myfone \circ \mv{h}_0 +  \myftwo \circ \Wy{S} \circ \Wy{S} \circ \myfone \circ \mv{h}_0 +  \myftwo \circ \myfone \circ \mv{h}_0 \\
  \myfthr \circ \myftwo \circ \Wy{S} \circ \myfone \circ \mv{h}_0 +  \myfthr \circ \myftwo \circ \myfone \circ \mv{h}_0 
      \end{matrix}
    \right]
  \end{equation}
In general, after the $k$-th iteration, if $S$ and $f_{\theta_i}$ are linear, with $k \ge 3$ we have
  \begin{equation} \label{eq:generalizations-diagonal-M3-iterationk}
    \circ_{i=1}^k M_{d}  
    \left(
      \begin{bmatrix}
          \mv{h}_0 \\
          0 \\
          0 \\
          0 \\
      \end{bmatrix}
      \right) = 
    \left[
      \begin{matrix}
  \mv{h}_0 \\
  ( \circ_{i=0}^{k-1} \Wy{S} ) \circ \myfone \circ \mv{h}_0 \\
  \myftwo \circ ( \circ_{i=0}^{k-2} \Wy{S} ) \circ \myfone \circ \mv{h}_0 \\
  \myfthr \circ \myftwo \circ ( \circ_{i=0}^{k-3} \Wy{S} ) \circ \myfone \circ \mv{h}_0 
      \end{matrix}
    \right]
  \end{equation}

So, in the linear case, the convergence of the above as $k \longmapsto \infty$ is determined by the convergence of the infinite product of $S$ alone, i.e., if we choose $S$ \emph{and} the $f_{\theta_j}$ to be a linear function  where the power-series is well understood.

%%%%%%%%%%%%%%%%%%%%%%%%%%%%%%%%%%%%%%%%%%%%%%%%%%%%%%%%%%%%%%%%%%%%%%%%
\subsection{Super-diagonal blocks} \label{sec:generalizations-superdiagonal}


Now consider
\begin{equation} \label{eq:generalizations-superdiagonal-M4}
  M_{ad} = 
    \left[
      \begin{matrix}
  \myI & 0 & 0 & 0\\
  \myfone & 0 & \myS & 0\\
  0 & \myftwo & 0 & 0\\
  0 & 0 & \myfthr & 0
      \end{matrix}
    \right]
  \end{equation}
  
  \begin{equation} \label{eq:generalizations-superdiagonal-M4-iteration3}
    \circ_{i=1}^{3}M_{ad}  
    \left(
      \begin{bmatrix}
          \mv{h}_0 \\
          0 \\
          0 \\
          0 \\
      \end{bmatrix}
      \right) = 
      \left[
      \begin{matrix}
  \mv{h}_0 \\
  \myfone \circ \mv{h}_0 + \myS \circ \myftwo \circ \myfone \circ \mv{h}_0 \\
  \myftwo \circ \myfone \circ \mv{h}_0 \\
  \myfthr \circ \myftwo \circ \myfone \circ \mv{h}_0 
      \end{matrix}
    \right]
  \end{equation}

\subsubsection{\tblue{Choice of the initial vector}}

\tblue{The iteration will {\bf not} be independent of the initial vector}

\begin{equation} \label{eq:generalizations-superdiagonal-M4-iteration3q}
    \circ_{i=1}^{3}M_{ad}  
    \left(
      \begin{bmatrix}
          \mv{h}_0 \\
          q_1 \\
          q_2 \\
          q_3 \\
      \end{bmatrix}
      \right) = 
      \left[
      \begin{matrix}
  \mv{h}_0 \\
  \myfone \circ \mv{h}_0 + \myS \circ \myftwo \circ \myfone \circ \mv{h}_0 + \myS \circ \myftwo \circ \myS \circ q_2 ) \\
  \myftwo \circ \myfone \circ \mv{h}_0 + \myftwo \circ \myS \circ \myftwo \circ q_1 \\
  \myfthr \circ \myftwo \circ \myfone \circ \mv{h}_0  + \myfthr \circ \myftwo \circ \myS \circ q_2
      \end{matrix}
    \right]
  \end{equation}

However, continuing from \eqref{eq:generalizations-superdiagonal-M4-iteration3} 
  
  \begin{equation} \label{eq:generalizations-superdiagonal-M4-iteration4}
    \circ_{i=1}^{4}M_{ad}  
    \left(
      \begin{bmatrix}
          \mv{h}_0 \\
          0 \\
          0 \\
          0 \\
      \end{bmatrix}
      \right) = 
    \left[
      \begin{matrix}
  \mv{h}_0 \\
  \left(\myS \circ \myftwo \circ \myfone \circ \mv{h}_0 +  \myfone \circ \mv{h}_0 \right) \\
  \left(\myftwo \circ \myS \circ \myftwo \circ \myfone \circ \mv{h}_0 +  \myftwo \circ \myfone \circ \mv{h}_0 \right) \\
  \myfthr \circ \myftwo \circ \myfone \circ \mv{h}_0 
      \end{matrix}
    \right]
  \end{equation}
  
  \begin{equation} \label{eq:generalizations-superdiagonal-M4-iteration5}
    \circ_{i=1}^{5}M_{ad}  
    \left(
      \begin{bmatrix}
          \mv{h}_0 \\
          0 \\
          0 \\
          0 \\
      \end{bmatrix}
      \right) = 
    \left[
      \begin{matrix}
  \mv{h}_0 \\
  \left(\myS \circ \myftwo \circ \myS \circ \myftwo \circ \myfone \circ \mv{h}_0 +  \myS \circ \myftwo \circ \myfone \circ \mv{h}_0 +  \myfone \circ \mv{h}_0 \right) \\
  \left(\myftwo \circ \myS \circ \myftwo \circ \myfone \circ \mv{h}_0 +  \myftwo \circ \myfone \circ \mv{h}_0 \right) \\
  \left(\myfthr \circ \myftwo \circ \myS \circ \myftwo \circ \myfone \circ \mv{h}_0 +  \myfthr \circ \myftwo \circ \myfone \circ \mv{h}_0 \right) 
      \end{matrix}
    \right]
  \end{equation}
  
  In general, after the $k$-th iteration, if $S$ and $f_{\theta_i}$ are linear, with $k$ odd and $k \ge 3$ we have

  \begin{equation} \label{eq:generalizations-superdiagonal-M4-iterationk-odd}
    \circ_{i=1}^{k} M_{ad}  
    \left(
      \begin{bmatrix}
          \mv{h}_0 \\
          0 \\
          0 \\
          0 \\
      \end{bmatrix}
      \right) = 
    \left[
      \begin{matrix}
  \mv{h}_0 \\
  ( \circ_{i=0}^{\frac{k-1}{2}} (\myS \circ \myftwo) ) \circ \myfone \circ \mv{h}_0 \\
  \myftwo \circ ( \circ_{i=0}^{\frac{k-3}{2}} (\myS \circ \myftwo) ) \circ \myfone \circ \mv{h}_0 \\
  \myfthr \circ \myftwo \circ ( \circ_{i=0}^{\frac{k-3}{2}} (\myS \circ \myftwo) ) \circ \myfone \circ \mv{h}_0 
      \end{matrix}
    \right]
  \end{equation}

After the $k$-th iteration, if $S$ and $f_{\theta_i}$ are linear, with $k$ even and $k \ge 4$ we have

  \begin{equation} \label{eq:generalizations-superdiagonal-M4-iterationk-even}
    \circ_{i=1}^{k} M_{ad}  
    \left(
      \begin{bmatrix}
          \mv{h}_0 \\
          0 \\
          0 \\
          0 \\
      \end{bmatrix}
      \right) = 
    \left[
      \begin{matrix}
  \mv{h}_0 \\
  ( \circ_{i=0}^{\frac{k-3}{2}} (\myS \circ \myftwo) ) \circ \myfone \circ \mv{h}_0 \\
  \myftwo \circ ( \circ_{i=0}^{\frac{k-3}{2}} (\myS \circ \myftwo) ) \circ \myfone \circ \mv{h}_0 \\
  \myfthr \circ \myftwo \circ ( \circ_{i=0}^{\frac{k-4}{2}} (\myS \circ \myftwo) ) \circ \myfone \circ \mv{h}_0 
      \end{matrix}
    \right]
  \end{equation}

So, in the liner case, the convergence of the above is determined by the convergence of the infinite product of $S \circ \myftwo$ alone!  Note, here $\myftwo$, and the $f_{\theta_j}$, are generally non-linear functions and the power-series is not available in closed form.  However, perhaps special cases of $f_{\theta_j}$ can be considered.

% \subsection{Top row of zeros} \label{sec:generalizations-RNN}

% Assigning zero blocks to the top row recalls the RNN \eqref{eq:RNN-dyamics}, i.e, 
% % Full matrix
% \begin{equation} \label{eq:generalizations-RNN}
%     \begin{bmatrix}
%         0 & 0  & 0  & 0  & 0 \\
%         \Wg{W_{2,1}} & \Wy{W_{2,2}}  & \Wr{W_{2,3}}  & \Wr{W_{2,4}}  & \Wr{W_{2,5}} \\
%         \Wb{W_{3,1}} & \Wg{W_{3,2}}  & \Wy{W_{3,3}}  & \Wr{W_{3,4}}  & \Wr{W_{3,5}} \\
%         \Wb{W_{4,1}} & \Wb{W_{4,2}}  & \Wg{W_{4,3}}  & \Wy{W_{4,4}}  & \Wr{W_{4,5}} \\
%         \Wb{W_{5,1}} & \Wb{W_{5,2}}  & \Wb{W_{5,3}}  & \Wg{W_{5,4}}  & \Wy{W_{5,5}} \\
%     \end{bmatrix}
%     =
%     \begin{bmatrix}
%         0 & 0 \\
%         W_1 & W_2 \\
%     \end{bmatrix}
% \end{equation}
% which is an RNN.
